# Supplementary material for: Unassisted Noise Reduction of Chemical Reaction Data Sets
Source: arXiv:2102.01399 source file (2021-02-02)

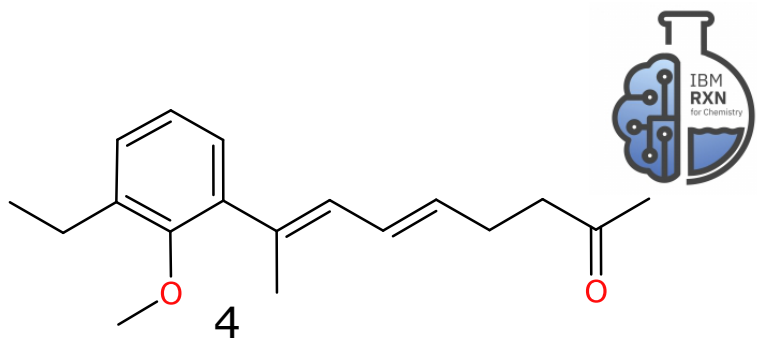

## Information about the retrosynthesis

Created On: 2020-05-18T15:27:05.381000

Model: 2020-04-24

Product: CC(CC/C=C/C=C(\C)/C1C(OC)=C(CC)C=CC=1)=O

MSSR: 10

FAP: 0.7

MRP: 20

SbP: 2

Available smiles:

Exclude smiles: CC(CC/C=C/C=C(\C)/C1C(OC)=C(CC)C=CC=1)=O

Exclude substructures:

Availability pricing threshold: 0

## Sequence 0, Confidence: 0.679

### Step 1

Type: Ketone Collins oxidation, Conf dence: 1.0

CCc1cccc(/C(C)=C/C=C/C/C(C)O)c1OC.ClCCl.O=[Cr](=O)([O-])Cl.c1cc[nH+]cc1>>CC(CC/C=C/C=C/C(C)OC)=C(CC)C=CC=1=O

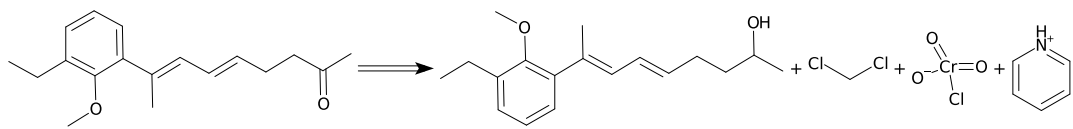

### Step 2

Type: Unrecognized, Conf dence: 1.0

CCc1cccc(/C(C)=C/C=C/C/C(C)O)c1OC.C1CCOC1.[Li]C>>CCc1cccc(/C(C)=C/C=C/C/C(C)O)c1OC

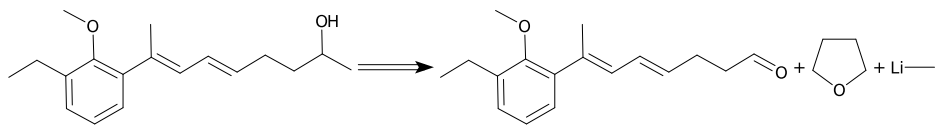

### Step 3

Type: Cyano to formyl, Conf dence: 0.997

CCc1cccc(/C(C)=C/C=C/C/C(C)O)c1OC.CC(C)C[AlH]CC(C)C.Cc1ccccc1.Cl>>CCc1cccc(/C(C)=C/C=C/C/C(C)O)c1OC

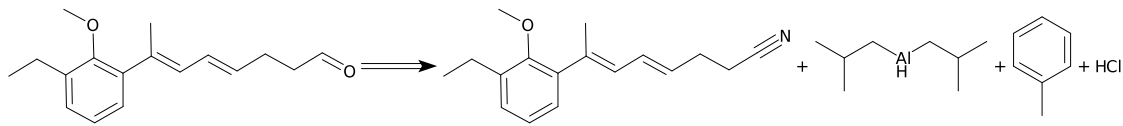

### Step 4

Type: Mesyloxy Kolbe nitrile synthesis, Conf dence: 1.0

CCc1cccc(/C(C)=C/C=C/C/C(C)O)c1OC.CN(C)C=O.[C-]#N.[Na+]>>CCc1cccc(/C(C)=C/C=C/C/C(C)O)c1OC

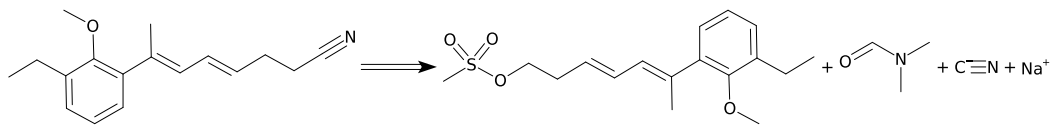

### Step 5

Type: Sulfonic ester Schotten-Baumann, Conf dence: 0.997

CCc1cccc(/C(C)=C/C=C/CCO)c1OC.C1CCOC1.CS(=O)(=O)Cl.O>>CCc1cccc(/C(C)=C/C=C/CCOS(C)(=O)=O)c1OC

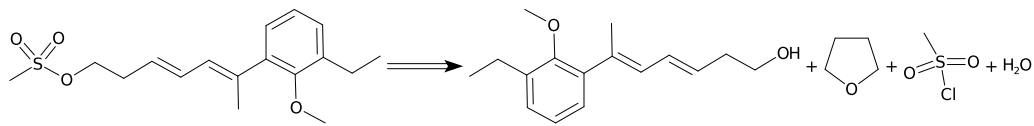

## Step 6

Type: Ester to alcohol reduction, Confidence: 0.897

CCOC(=O)C/C=C/C=C(\C)c1cccc(CC)c1OC.CC(C)C[AlH]CC(C)C>>CCc1cccc(/C(C)=C/C=C/CCO)c1OC

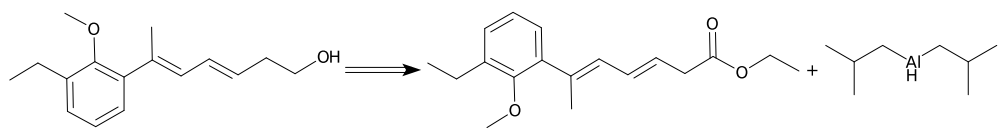

## Step 7

Type: Horner-Wadsworth-Emmons reaction, Confidence: 0.773

CCOC(=O)C/C=C/C/CP(=O)(OCC)OCC.CCc1cccc(C(C)=O)c1OC.COCCOC.[NaH]>>CCOC(=O)C/C=C/C=C(\C)c1cccc(CC)c1OC

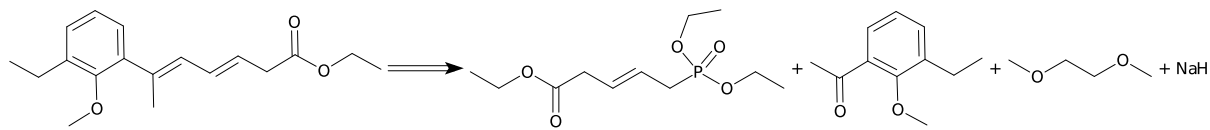

## Step 8

Type: Michaelis-Arbuzov reaction, Confidence: 1.0

CCOC(=O)C/C=C/C/CBr.CC#N.CCOP(=O)(OCC)OCC>>CCOC(=O)C/C=C/C/CP(=O)(OCC)OCC

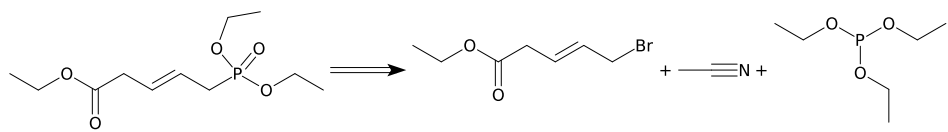

Type: Alcohol to ketone oxidation, Confidence: 1.0

CCc1cccc(C(C)O)c1OC.ClCCl.O=[Mn]=O>>CCc1cccc(C(C)=O)c1OC

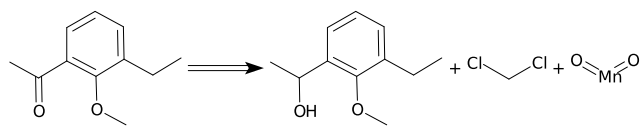

## Step 9

**Type: Fischer-Speier esterification, Confidence: 1.0**

O=C(O)C/C=C/CBr.CCO.O=S(=O)(O)O>>CCOC(=O)C/C=C/CBr

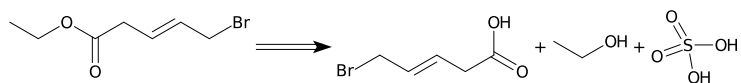

**Type: Unrecognized, Confidence: 1.0**

CCc1cccc(C=O)c1OC.C1CCOC1.[Li]C>>CCc1cccc(C(C)O)c1OC

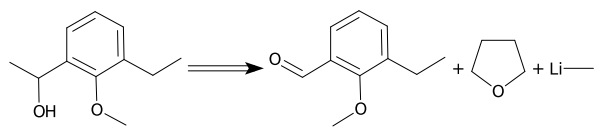

## Step 10

**Type: Wohl-Ziegler bromination, Confidence: 0.985**

C/C=C/CC(=O)O.ClC(Cl)(Cl)Cl.O=C1CCC(=O)N1Br>>O=C(O)C/C=C/CBr

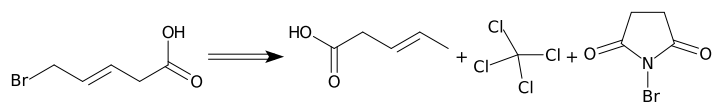

**Type: Hydroxy to methoxy, Confidence: 1.0**

CCc1cccc(C=O)c1O.Cl>>CCc1cccc(C=O)c1OC

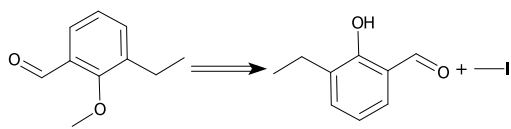

Supplement: Supplementary file 1 [file c4_seq0_final.pdf]
