# Supplementary material for: Unassisted Noise Reduction of Chemical Reaction Data Sets
Source: arXiv:2102.01399 source file (2021-02-02)

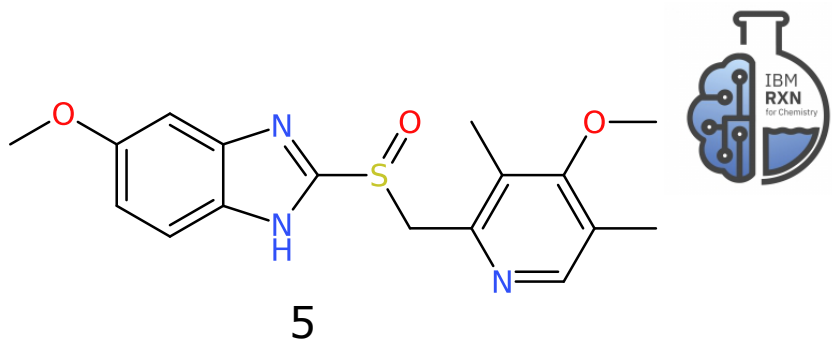

## Information about the retrosynthesis

Created On: 2020-05-28T08:58:05.020000

Model: 2020-04-24

Product: COC1C=CC2=C(N=C(N2)S(=O)CC2N=CC(C)=C(OC)C=2C)C=1

MSSR: 10

FAP: 0.7

MRP: 20

SbP: 2

Available smiles:

Exclude smiles: COC1ccc2[nH]c(SCc3ncc(C)c(OC)c3C)nc2c1, COC1c(C)cnc(CCl)c1C, COC1ccc2[nH]c(S)nc2c1, COC1C=CC2=C(N=C(N2)S(=O)CC2N=CC(C)=C(OC)C=2C)C=1

Exclude substructures:

Availability pricing threshold: 0

## Sequence 0, Confidence: 0.823

### Step 1

Type: Sulfanyl to sulfinyl, Confidence: 0.922

COc1ccc2[nH]c(SCc3ncc(C)c(OC)c3C)nc2c1>>COC1C=CC2=C(N=C(N2)S(=O)CC2N=CC(C)=C(OC)C=2C)C=1

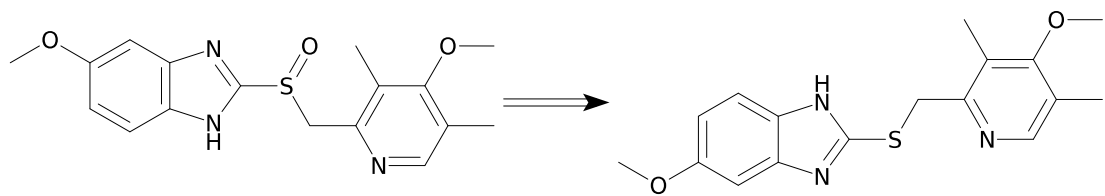

### Step 2

Type: Thioether synthesis, Confidence: 0.999

COc1c(C)cnc(CCl)c1C.COc1ccc2[nH]c(S)nc2c1>>COc1ccc2[nH]c(SCc3ncc(C)c(OC)c3C)nc2c1

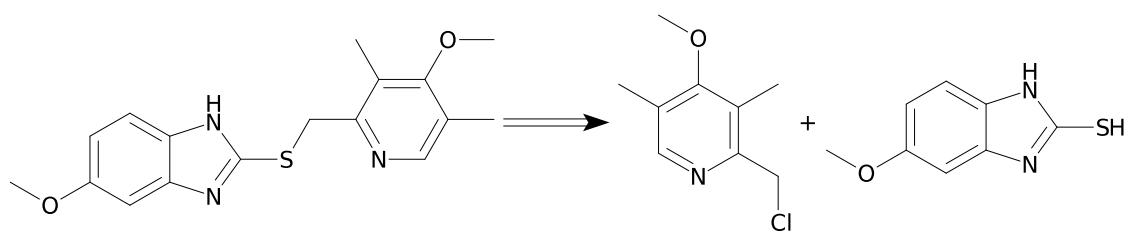

### Step 3

Type: Hydroxy to chloro, Confidence: 1.0

COc1c(C)cnc(CO)c1C.ClCCl.O=S(Cl)Cl.O.O.O.O>>COc1c(C)cnc(CCl)c1C

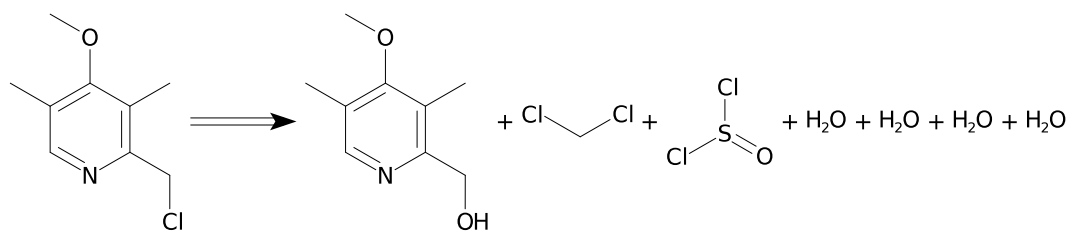

Type: Benzimidazolethione synthesis, Confidence: 0.894

CCO.COc1ccc(N)c(N)c1.S=C=S.[K+].[OH-].[K+].[OH-]>>COc1ccc2[nH]c(S)nc2c1

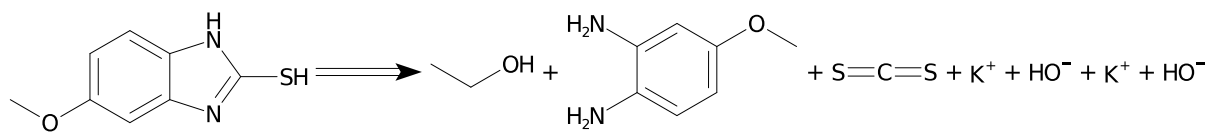

Supplement: Supplementary file 2 [file c5_seq0_final.pdf]
