# Supplementary material for: Unassisted Noise Reduction of Chemical Reaction Data Sets
Source: arXiv:2102.01399 source file (2021-02-02)

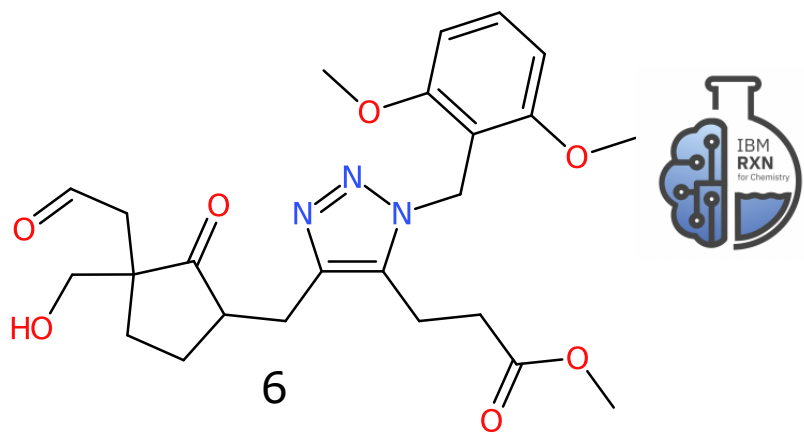

## Information about the retrosynthesis

Created On: 2020-05-19T07:38:18.454000

Model: 2020-04-24

Product: COC(=O)CCC1=C(CC2CCC(CO)(CC=O)C2=O)N=NN1CC1C(OC)=CC=CC=1OC

MSSR: 10

FAP: 0.7

MRP: 20

SbP: 2

Available smiles:

Exclude smiles: COC(=O)CCC1=C(CC2CCC(CO)(CC=O)C2=O)N=NN1CC1C(OC)=CC=CC=1OC

Exclude substructures:

Availability pricing threshold: 0

## Sequence 0, Confidence: 0.965

### Step 1

Type: Ozonolysis, Conf dence: 0.985

C=CCC1(CO)CCC(Cc2nnn(Cc3c(OC)cccc3OC)c2CCC(=O)OC)C1=O.CO.CSC.ClCCl.O=[O+][O-]>>COC(=O)CCC1=C(CC2CCC(CO)(CC=O)C2=O)N=NN1CC1C(OC)=CC=CC=1OC

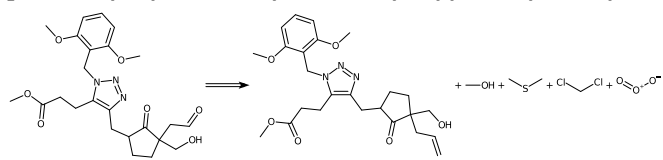

### Step 2

Type: O-THP deprotection, Conf dence: 0.998

C=CCC1(COC2CCCCO2)CCC(Cc2nnn(Cc3c(OC)cccc3OC)c2CCC(=O)OC)C1=O.CO.Cc1ccc(S(=O)(=O)[O-])cc1.c1cc[nH+]cc1>>C=CCC1(CO)CCC(Cc2nnn(Cc3c(OC)cccc3OC)c2CCC(=O)OC)C1=O

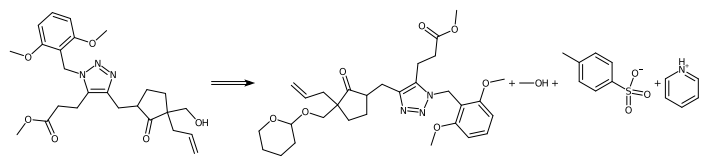

### Step 3

Type: Unrecognized, Conf dence: 0.988

C=CCC1(COC2CCCCO2)CCCC1=O.CO.CC(=O)CCc1c(Cl)nnn1Cc1c(OC)cccc1OC.C1CCOC1.C[Si](C)(C)[N-][Si](C)(C)C.[Li+]>>C=CCC1(COC2CCCCO2)CCC(Cc2nnn(Cc3c(OC)cccc3OC)c2CCC(=O)OC)C1=O

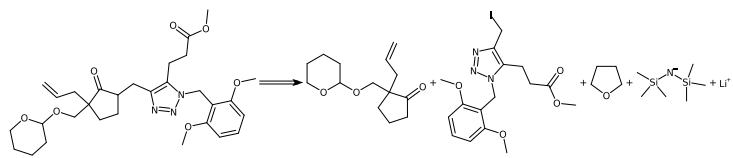

### Step 4

Type: Unrecognized, Conf dence: 0.998

O=C1CCCC1COC1CCCCO1.C=CCBr.CN(C)C=O.[H-].[Na+]>>C=CCC1(COC2CCCCO2)CCCC1=O

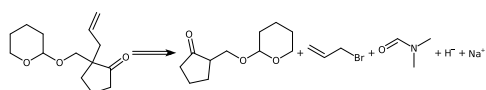

Type: Hydroxy to iodo, Confidence: 1.0

COC(=O)CCc1c(CO)nnn1Cc1c(OC)cccc1OC.II.c1c[nH]cn1.c1ccc(P(c2ccccc2)c2ccccc2)cc1>>COC(=O)CCc1c(Cl)nnn1Cc1c(OC)cccc1OC

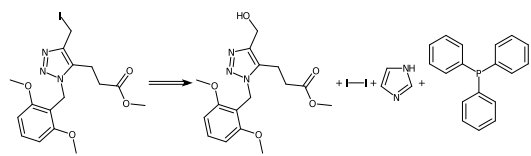

## Step 5

Type: Alkene ether synthesis, Confidence: 1.0

C1=COCCC1.ClCCl.O=C1CCCC1CO>>O=C1CCCC1COC1CCCCO1

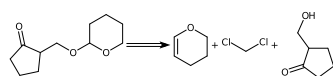

Type: Alkene hydrogenation, Confidence: 0.999

COC(=O)/C=C/c1c(CO)nnn1Cc1c(OC)cccc1OC.CO.[H][H].[Pd]>>COC(=O)CCc1c(CO)nnn1Cc1c(OC)cccc1OC

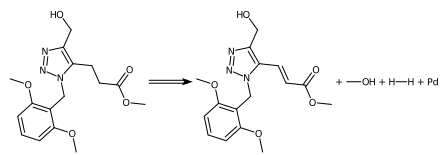

## Step 6

Type: O-TBS deprotection, Confidence: 1.0

COC(=O)/C=C/c1c(CO[Si](C)(C)C(C)(C)C)nnn1Cc1c(OC)cccc1OC.C1CCOC1.F.c1ccncc1>>CO C(=O)/C=C/c1c(CO)nnn1Cc1c(OC)cccc1OC

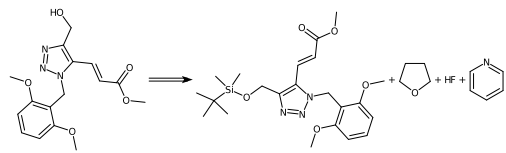

## Step 7

Type: Horner-Wadsworth-Emmons reaction, Confidence: 0.997

COc1cccc(OC)c1Cn1nnc(CO[Si](C)(C)C(C)(C)C)c1C=O.C1CCOC1.CCOP(=O)(CC(=O)OC)OCC.[H-].[Na+]>>COC(=O)/C=C/c1c(CO[Si](C)(C)C(C)(C)C)nnn1Cc1c(OC)cccc1OC

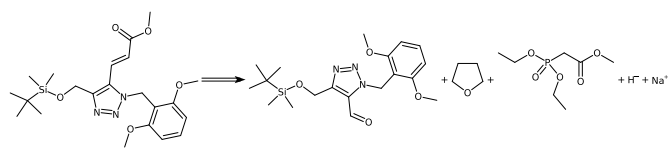

## Step 8

Type: Vilsmeier-Haack reaction, Confidence: 0.999

COc1cccc(OC)c1Cn1cc(CO[Si](C)(C)C(C)(C)C)nn1.C1CCOC1.CN(C)C=O.[Li]CCCC>>COc1cc  
cc(OC)c1Cn1nnc(CO[Si](C)(C)C(C)(C)C)c1C=O

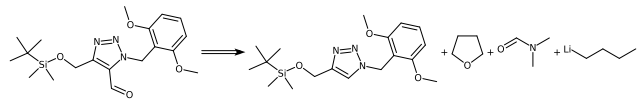

## Step 9

Type: O-TBS protection, Confidence: 1.0

COc1cccc(OC)c1Cn1cc(CO)nn1.CC(C)(C)[Si](C)(C)Cl.CN(C)C=O.O.c1c[nH]cn1>>COc1cccc(OC)c1Cn1cc(CO[Si](C)(C)C(C)(C)C)nn1

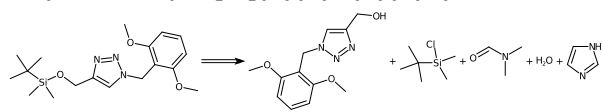

## Step 10

Type: Azide-alkyne Huisgen cycloaddition, Confidence: 1.0

C#CCO.COc1cccc(OC)c1CN=[N+]=[N-].O.O=C1O[C@H]([C@@H](O)CO)C([O-])=C1O.[Na+].O.O.O.O.O=S(=O)([O-])[O-].[Cu+2].O=C1O[C@H]([C@@H](O)CO)C([O-])=C1O.[Na+].O.O.O.O.O.O=S(=O)([O-])[O-].[Cu+2]>>COc1cccc(OC)c1Cn1cc(CO)nn1

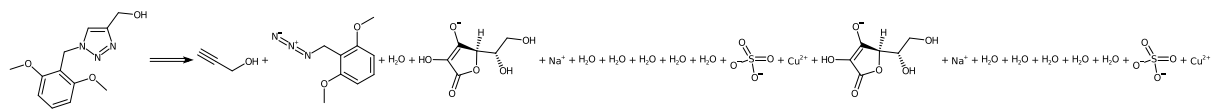

Supplement: Supplementary file 3 [file c6_seq0_final.pdf]
