# Supplementary material for: Unassisted Noise Reduction of Chemical Reaction Data Sets
Source: arXiv:2102.01399 source file (2021-02-02)

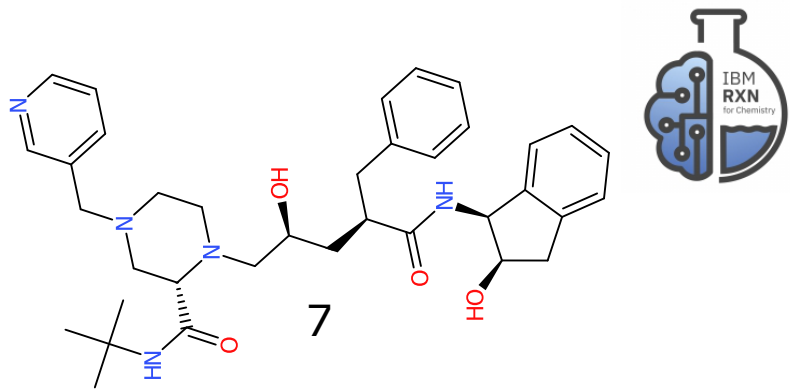

## Information about the retrosynthesis

Created On: 2020-05-29T16:24:15.866000

Model: 2020-04-24

Product: C1C=C2C(C[C@H]([C@H]2NC([C@@H](C[C@@H](CN2[C@H](C(NC(C)(C)C)=O)CN(C(C3C=CC=NC=3)CC2)O)CC2C=CC=CC=2)=O)O)=CC=1

MSSR: 10

FAP: 0.7

MRP: 20

SbP: 2

Available smiles:

Exclude smiles: C1C=C2C(C[C@H]([C@H]2NC([C@@H](C[C@@H](CN2[C@H](C(NC(C)(C)C)=O)CN(C(C3C=CC=NC=3)CC2)O)CC2C=CC=CC=2)=O)O)=CC=1, C1C=C2C(C[C@H]([C@H]2NC([C@@H](C[C@@H](CN2[C@H](C(NC(C)(C)C)=O)CN(C(C3C=CC=NC=3)CC2)O)CC2C=CC=CC=2)=O)O)=CC=1

Exclude substructures:

Availability pricing threshold: 0

## Sequence 0, Confidence: 0.896

### Step 1

Type: Chloro N-alkylation, Confidence: 0.988

CC(C)(C)NC(=O)[C@@H]1CNCCN1C[C@@H](O)C[C@@H](Cc1ccccc1)C(=O)N[C@H]1c2ccccc2C[C@H]1O.CN(C)C=O.ClCc1ccncc1>>C1C=C2C(C[C@H]([C@H]2NC([C@@H](C[C@@H](C N2[C@H](C(NC(C)(C)C)=O)CN(CC3C=CC=NC=3)CC2)O)CC2C=CC=CC=2)=O)O)=CC=1

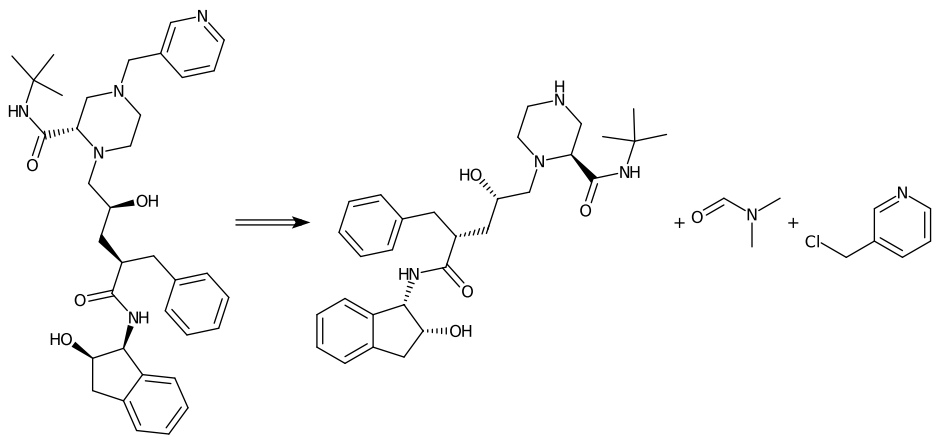

### Step 2

Type: N-Bn deprotection, Confidence: 1.0

CC(C)(C)NC(=O)[C@@H]1CN(Cc2ccccc2)CCN1C[C@@H](O)C[C@@H](Cc1ccccc1)C(=O)N[C@H]1c2ccccc2C[C@H]1O.CO.[Pd]>>CC(C)(C)NC(=O)[C@@H]1CNCCN1C[C@@H](O)C[C@@H](Cc1ccccc1)C(=O)N[C@H]1c2ccccc2C[C@H]1O

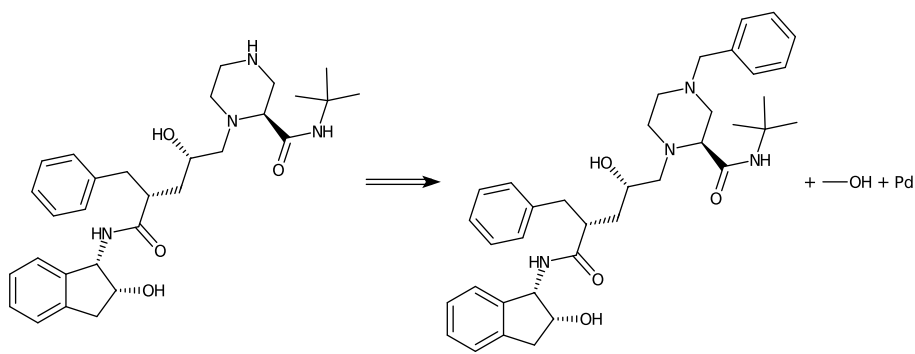

### Step 3

Type: Carboxylic acid + amine condensation, Confidence: 0.986

CC(C)(C)NC(=O)[C@@H]1CN(Cc2ccccc2)CCN1C[C@@H](O)C[C@@H](Cc1ccccc1)C(=O)O.N[C@H]1c2ccccc2C[C@H]1O>>CC(C)(C)NC(=O)[C@@H]1CN(Cc2ccccc2)CCN1C[C@@H](O)C[C@@H](Cc1ccccc1)C(=O)N[C@H]1c2ccccc2C[C@H]1O

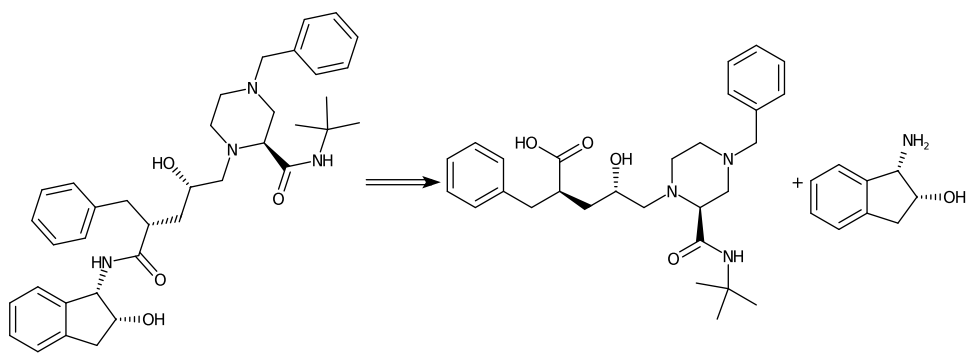

## Step 4

Type: Ester hydrolysis, Confidence: 0.932

CC(C)(C)NC(=O)[C@@H]1CN(Cc2ccccc2)CCN1C[C@@H]1C[C@@H](Cc2ccccc2)C(=O)O1.C  
O.O[Na]>>CC(C)(C)NC(=O)[C@@H]1CN(Cc2ccccc2)CCN1C[C@@H](O)C[C@@H](Cc1ccccc1)  
C(=O)O

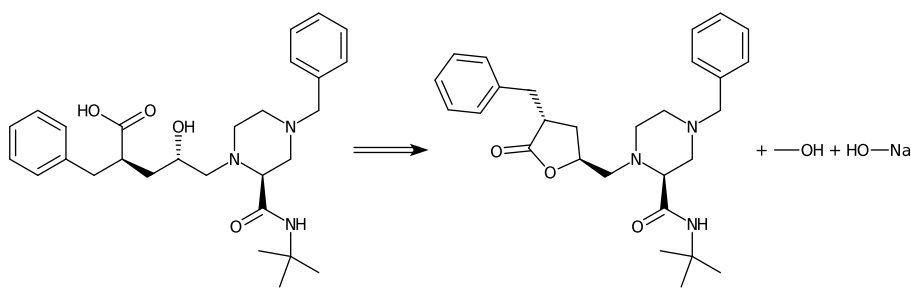

## Step 5

Type: Unrecognized, Confidence: 0.996

CC(C)(C)NC(=O)[C@@H]1CN(Cc2ccccc2)CCN1C[C@@H]1CCC(=O)O1.BrCc1ccccc1.C1CCO  
C1.C[Si](C)(C)[N-][Si](C)(C)C.[Li+]>>CC(C)(C)NC(=O)[C@@H]1CN(Cc2ccccc2)CCN1C[C@@H]  
1C[C@@H](Cc2ccccc2)C(=O)O1

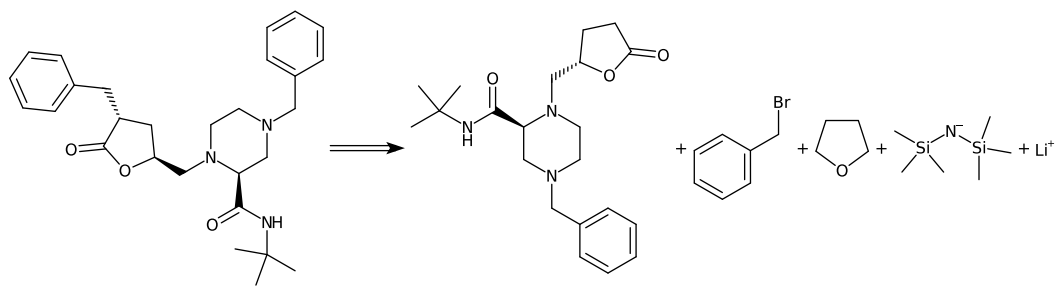

## Step 6

Type: Tosyloxy N-alkylation, Confidence: 0.999

CC(C)(C)NC(=O)[C@@H]1CN(Cc2ccccc2)CCN1.CC#N.Cc1ccc(S(=O)(=O)OC[C@@H]2CCC(=  
O)O2)cc1.O=C([O-])[O-].[K+].[K+]>>CC(C)(C)NC(=O)[C@@H]1CN(Cc2ccccc2)CCN1C[C@@H]  
1CCC(=O)O1

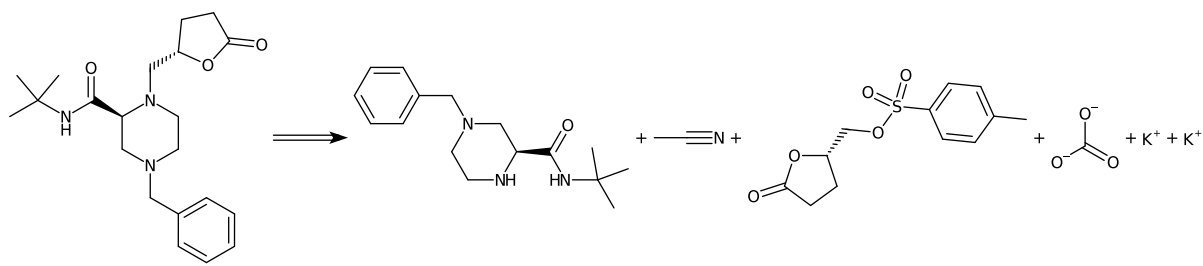

## Step 7

Type: N-Boc deprotection, Confidence: 0.999

CC(C)(C)NC(=O)[C@@H]1CN(Cc2ccccc2)CCN1C(=O)OC(C)(C)C.C1COCCO1.Cl.CICCl>>CC(C)(C)NC(=O)[C@@H]1CN(Cc2ccccc2)CCN1

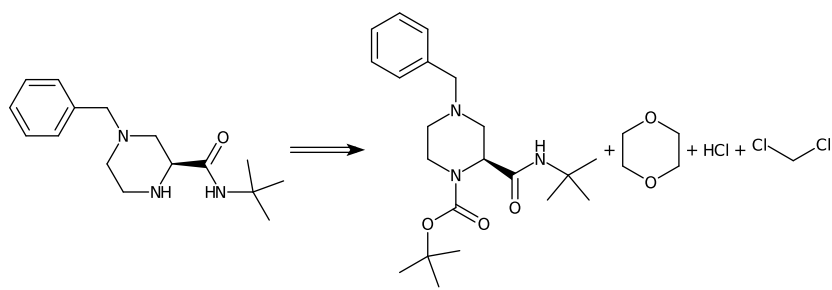

## Step 8

Type: Carboxylic acid + amine condensation, Confidence: 0.993

CC(C)(C)OC(=O)N1CCN(Cc2ccccc2)C[C@H]1C(=O)O.CC(C)(C)N.CCN(C(C)C)C(C)C.CN(C)C=O.CICCCl.On1nnc2ccccc21>>CC(C)(C)NC(=O)[C@@H]1CN(Cc2ccccc2)CCN1C(=O)OC(C)(C)C

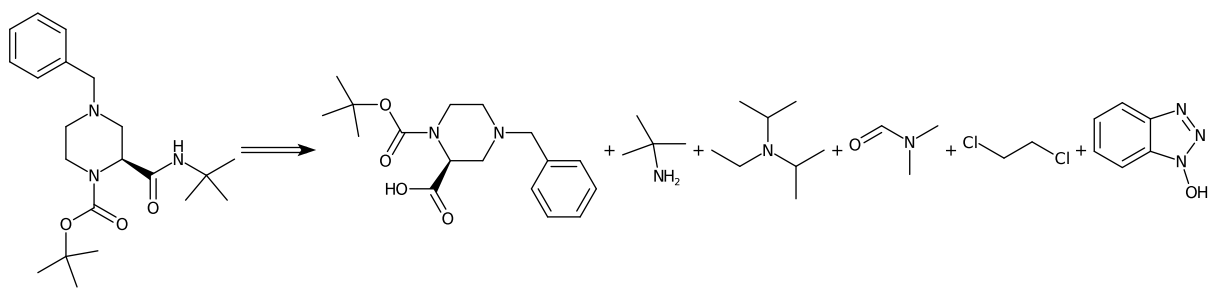

## Step 9

Type: N-Boc protection, Confidence: 1.0

C1COCCO1.CC(C)(C)OC(=O)OC(=O)OC(C)(C)C.O=C(O)[C@@H]1CN(Cc2ccccc2)CCN1.O[Na]>>CC(C)(C)OC(=O)N1CCN(Cc2ccccc2)C[C@H]1C(=O)O

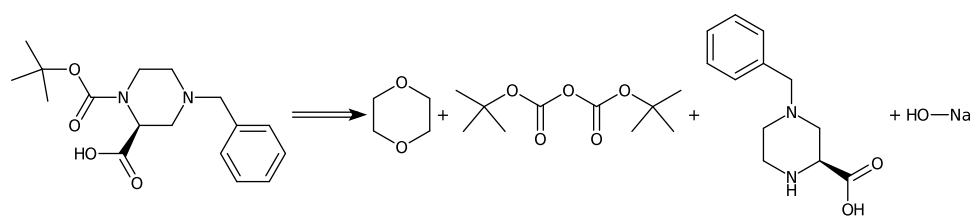

Supplement: Supplementary file 4 [file c7_seq0_excluded_final.pdf]
