# Supplementary material for: Unassisted Noise Reduction of Chemical Reaction Data Sets
Source: arXiv:2102.01399 source file (2021-02-02)

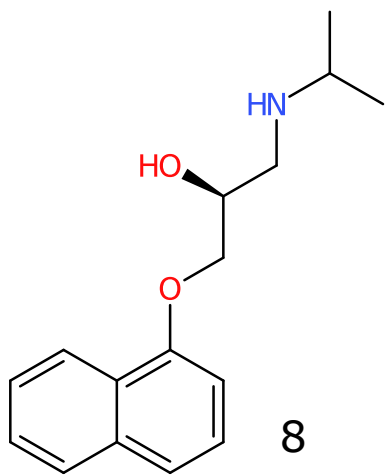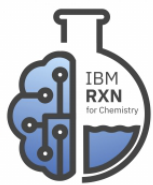

## Information about the retrosynthesis

Created On: 2020-05-28T09:06:21.924000

Model: 2020-04-24

Product: C1C2C(=CC=CC=2OC[C@H](CNC(C)C)O)C=CC=1

MSSR: 10

FAP: 0.7

MRP: 20

SbP: 2

Available smiles:

Exclude smiles: C1C2C(=CC=CC=2OC[C@@H]2CO2)C=CC=1,

C1C2C(=CC=CC=2OC[C@H](CNC(C)C)O)C=CC=1

Exclude substructures:

Availability pricing threshold: 0

## Sequence 1, Confidence: 0.996

### Step 1

Type: Unrecognized, Confidence: 0.996

CC(C)N1C[C@@H](COc2cccc3ccccc23)OC1=O.CO.O[Na]>>C1C2C(=CC=CC=2OC[C@H](CN(C)C)O)C=CC=1

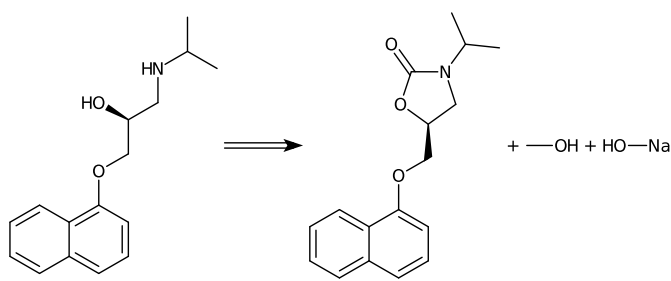

### Step 2

Type: Mitsunobu aryl ether synthesis, Confidence: 1.0

CC(C)N1C[C@@H](CO)OC1=O.C1CCOC1.CCOC(=O)N=NC(=O)OCC.Oc1cccc2ccccc12.c1ccc(P(c2ccccc2)c2ccccc2)cc1>>CC(C)N1C[C@@H](COc2cccc3ccccc23)OC1=O

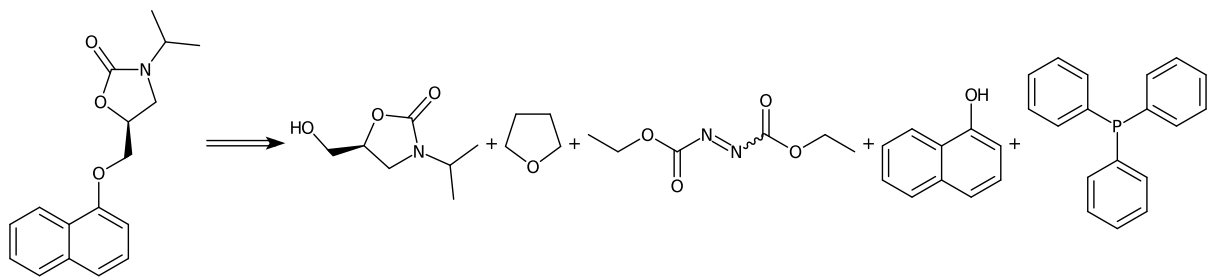

### Step 3

Type: O-TBS deprotection, Confidence: 1.0

CC(C)N1C[C@@H](CO[Si](C)(C)C(C)(C)C)OC1=O.C1CCOC1.CCCC[N+](CCCC)(CCCC)CCCC.[F-]>>CC(C)N1C[C@@H](CO)OC1=O

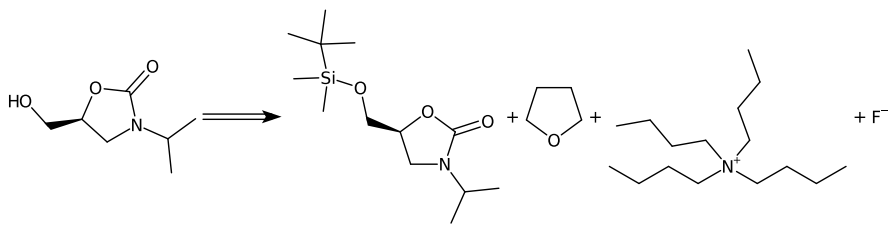

### Step 4

Type: Iodo N-alkylation, Confidence: 1.0

CC(C)(C)[Si](C)(C)OC[C@H]1CNC(=O)O1.C1CCOC1.CC(C)I.CCOC(C)=O.O.[NaH]>>CC(C)N1C[C@H](CO[Si](C)(C)C(C)(C)C)OC1=O

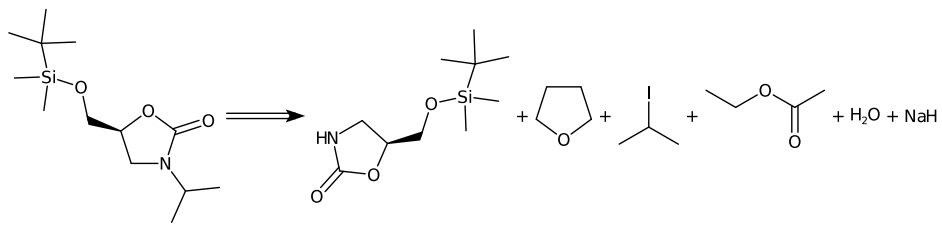

## Step 5

Type: O-TBS protection, Confidence: 1.0

CC(C)(C)[Si](C)(C)Cl.CCOC(C)=O.CN(C)C=O.O=C1NC[C@H](CO)O1>>CC(C)(C)[Si](C)(C)OC[C@H]1CNC(=O)O1

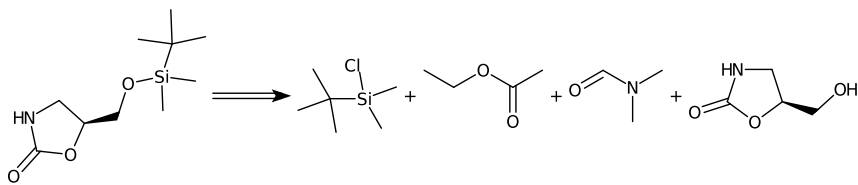

Supplement: Supplementary file 5 [file c8_seq1_final.pdf]
