# Supplementary material for: Unassisted Noise Reduction of Chemical Reaction Data Sets
Source: arXiv:2102.01399 source file (2021-02-02)

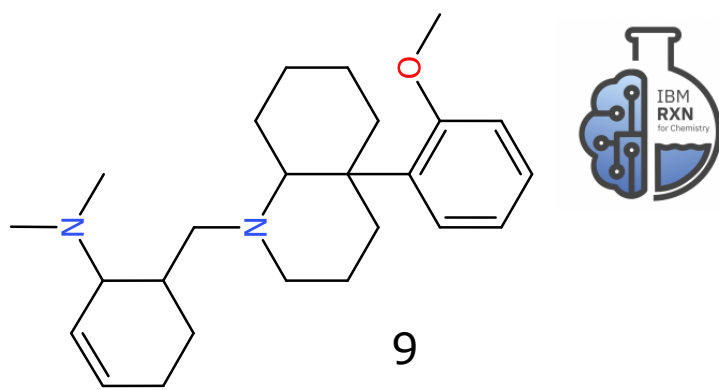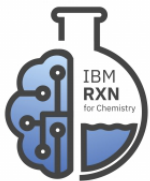

## Information about the retrosynthesis

Created On: 2020-05-19T14:34:34.406000

Model: 2020-04-24

Product: C1CC2(C(CCCC2)N(CC2CCC=CC2N(C)C)C1)C1C=CC=CC=1OC

MSSR: 10

FAP: 0.7

MRP: 20

SbP: 2

Available smiles:

Exclude smiles: C1CC2(C(CCCC2)N(CC2CCC=CC2N(C)C)C1)C1C=CC=CC=1OC

Exclude substructures:

Availability pricing threshold: 0

## Sequence 0, Confidence: 0.534

### Step 1

Type: Aldehyde reductive amination, Conf dence: 0.997

CN(C)C1C=CCCC1C=O.COc1ccccc1C12CCCCC1NCCC2.CC(=O)O[BH-](OC(C)=O)OC(C)=O.[Na+].ClCCl>>C1CC2(C(CCCC2)N(CC2CCC=CC2N(C)C)C1)C1C=CC=CC=1OC

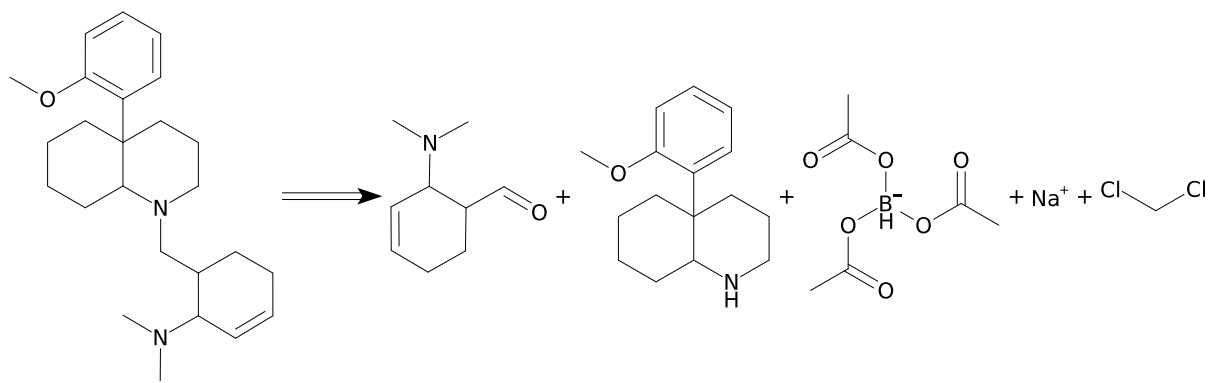

### Step 2

Type: Aldehyde Swern oxidation, Conf dence: 1.0

CN(C)C1C=CCCC1CO.CS(C)=O.ClCCl.O=C(Cl)C(=O)Cl>>CN(C)C1C=CCCC1C=O

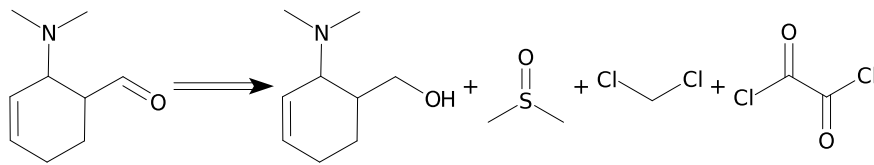

Type: Secondary ketimine reduction, Conf dence: 0.976

COc1ccccc1C12CCCCC1=NCCC2.CC[SiH](CC)CC.O=C(O)C(F)(F)F>>COc1ccccc1C12CCCCC1NCCC2

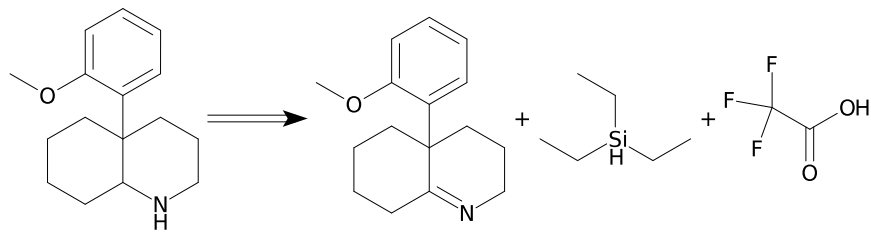

### Step 3

Type: Ester to alcohol reduction, Conf dence: 0.999

COC(=O)C1CCC=CC1N(C)C.C1CCOC1.O.[AlH4-].[Li+]>>CN(C)C1C=CCCC1CO

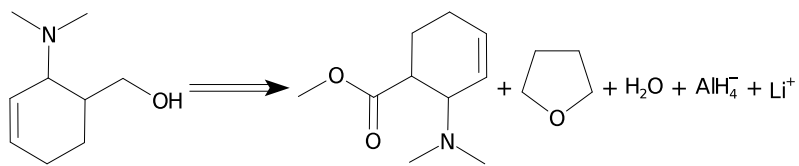

**Type:** Alkylimino-de-oxo-bisubstitution, **Confidence:** 0.567

COc1ccccc1C1(CCCN)CCCCC1=O.Cc1ccc(S(=O)(=O)O)cc1.Cc1ccccc1>>COc1ccccc1C12CC  
CCC1=NCCC2

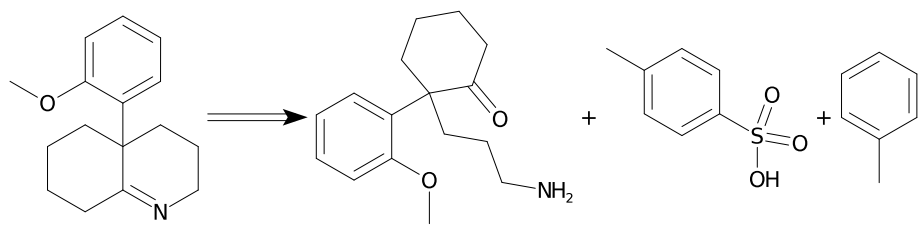

#### Step 4

**Type:** Methyl esterification, **Confidence:** 0.999

CN(C)C1C=CCCC1C(=O)O.CO.O=S(Cl)Cl>>COC(=O)C1CCC=CC1N(C)C

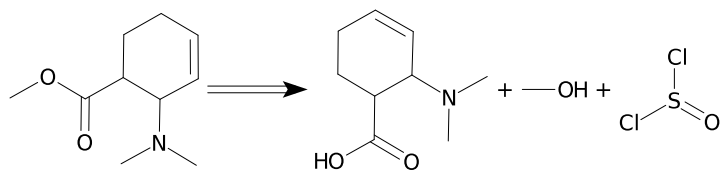

**Type:** N-Phth deprotection, **Confidence:** 0.975

COc1ccccc1C1(CCCN2C(=O)c3ccccc3C2=O)CCCCC1=O>>COc1ccccc1C1(CCCN)CCCCC1=O

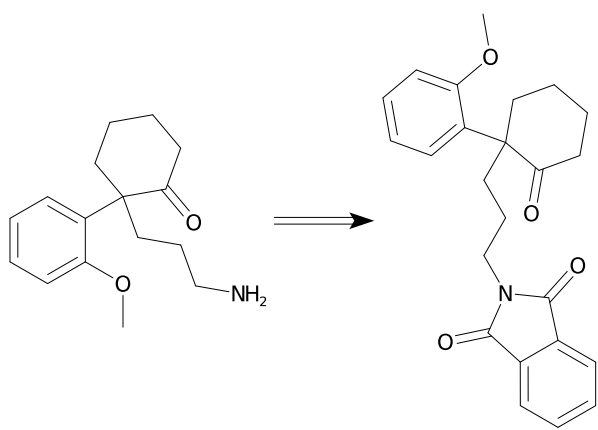

#### Step 5

Type: CO<sub>2</sub>H-Et deprotection, Confidence: 1.0

CCOC(=O)C1CCC=CC1N(C)C.CCO.O[Na]>>CN(C)C1C=CCCC1C(=O)O

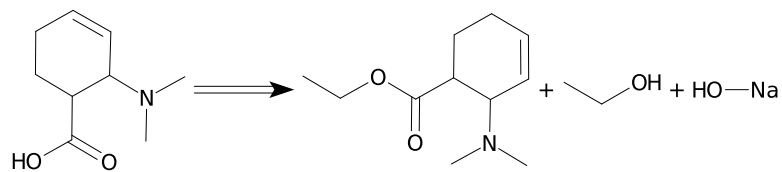

Type: Chloro Gabriel alkylation, Confidence: 1.0

COc1ccccc1C1(CCCCl)CCCCC1=O.CN(C)C=O.O=C1NC(=O)c2ccccc21.[K]>>COc1ccccc1C1(CCCN2C(=O)c3ccccc3C2=O)CCCCC1=O

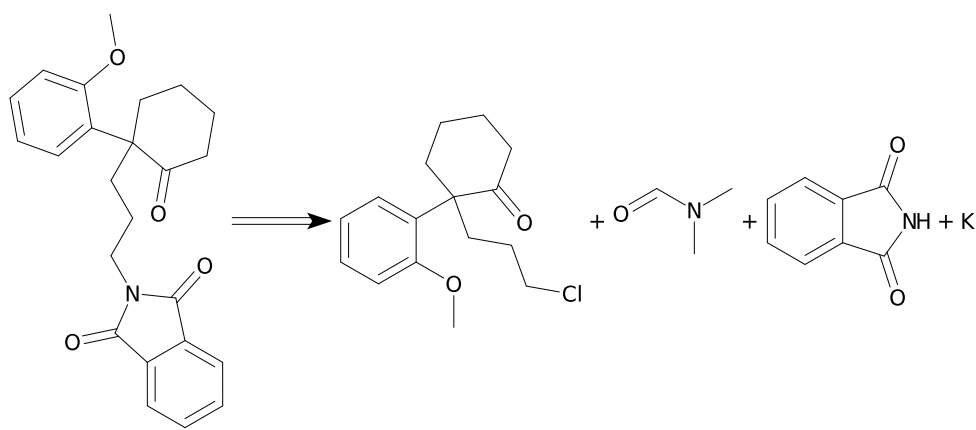

## Step 6

Type: N-methylation, Confidence: 0.999

CCOC(=O)C1CCC=CC1N.C=O.CC(=O)O.CO.[BH3-]C#N.[Na+]>>CCOC(=O)C1CCC=CC1N(C)C

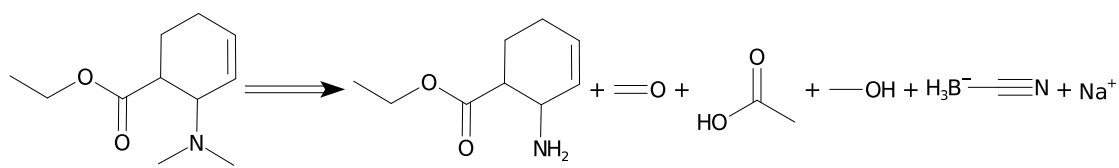

Type: Unrecognized, Confidence: 0.998

COc1ccccc1C1CCCCC1=O.CN(C)C=O.ClCCCl.[H-].[Na+]>>COc1ccccc1C1(CCCCl)CCCCC1=O

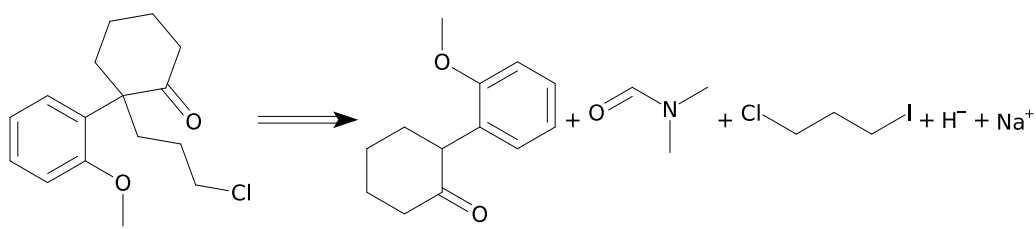

## Step 7

Type: Fischer-Speier esterification, Confidence: 0.998

CCO.NC1C=CCCC1C(=O)O.O=S(=O)(O)O>>CCOC(=O)C1CCC=CC1N

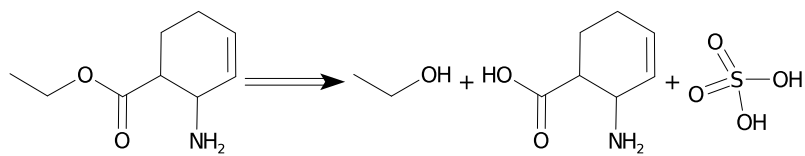

Type: Bromo Suzuki-type coupling, Confidence: 0.999

COc1ccccc1B(O)O.O=C1CCCCC1Br>>COc1ccccc1C1CCCCC1=O

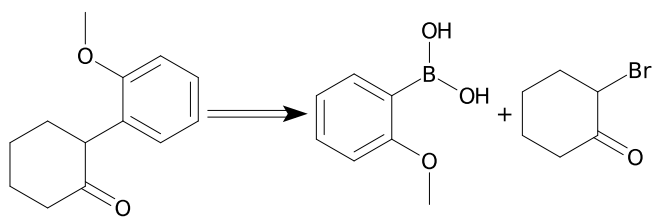

Supplement: Supplementary file 6 [file c9_seq0_final.pdf]
