# Supplementary material for: Unassisted Noise Reduction of Chemical Reaction Data Sets
Source: arXiv:2102.01399 source file (2021-02-02)

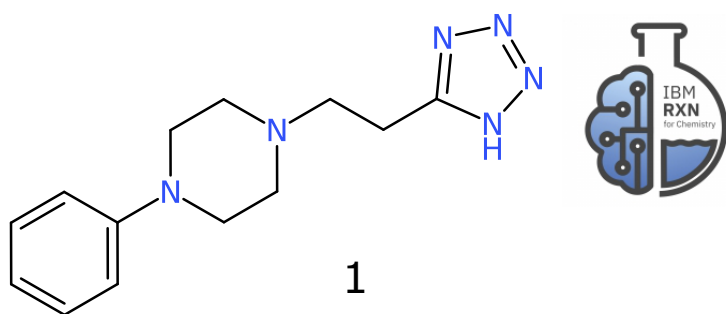

## Information about the retrosynthesis

Created On: 2020-05-18T15:03:44.351000

Model: 2020-04-24

Product: C1C(N2CCN(CCC3NN=NN=3)CC2)=CC=CC=1

MSSR: 10

FAP: 0.7

MRP: 20

SbP: 2

Available smiles:

Exclude smiles: C1C=CC(N2CCN(CCC3=NN=NN3)CC2)=CC=1,

C1C(N2CCN(CCC3NN=NN=3)CC2)=CC=CC=1

Exclude substructures:

Availability pricing threshold: 0

## Sequence 0, Confidence: 1.0

### Step 1

Type: Unrecognized, Confidence: 1.0

C=Cc1nn[nH]1.CCO.c1ccc(N2CCNCC2)cc1>>C1C(N2CCN(CCC3NN=NN=3)CC2)=CC=CC=1

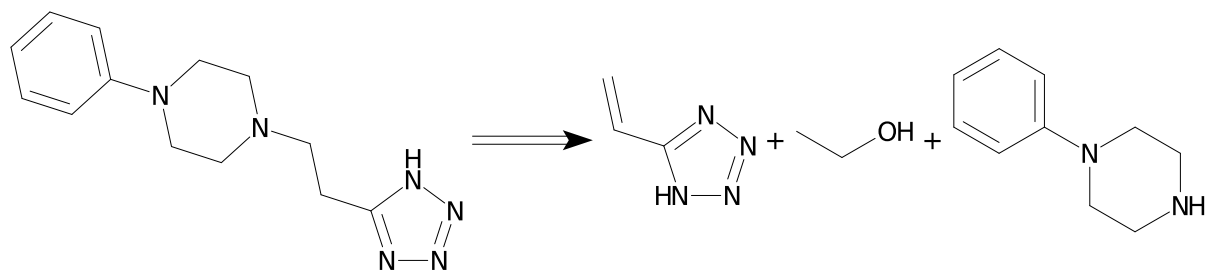

Supplement: Supplementary file 7 [file c1_seq0_final.pdf]
