# Supplementary material for: Unassisted Noise Reduction of Chemical Reaction Data Sets
Source: arXiv:2102.01399 source file (2021-02-02)

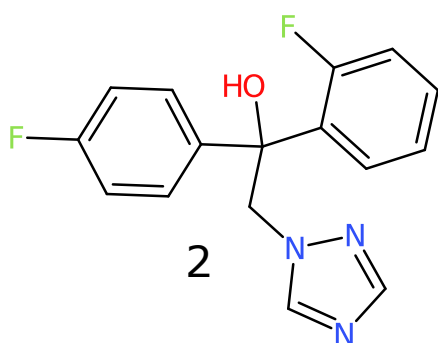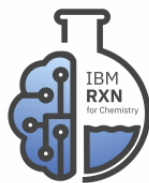

## Information about the retrosynthesis

Created On: 2020-05-18T15:12:49.268000

Model: 2020-04-24

Product: N1(N=CN=C1)CC(C1C=CC=CC=1F)(C1C=CC(F)=CC=1)O

MSSR: 10

FAP: 0.7

MRP: 20

SbP: 2

Available smiles:

Exclude smiles: N(CC(O)(C1=CC=C(F)C=C1)C1C(F)=CC=CC=1)1C=NC=N1,

N1(N=CN=C1)CC(C1C=CC=CC=1F)(C1C=CC(F)=CC=1)O

Exclude substructures:

Availability pricing threshold: 0

## Sequence 0, Confidence: 0.998

### Step 1

Type: Bromo Grignard reaction, Confidence: 0.999

O=C(Cn1cncn1)c1ccccc1F.C1CCOC1.Fc1ccc([Mg]Br)cc1>>N1(N=CN=C1)CC(C1C=CC=CC=1F)(C1C=CC(F)=CC=1)O

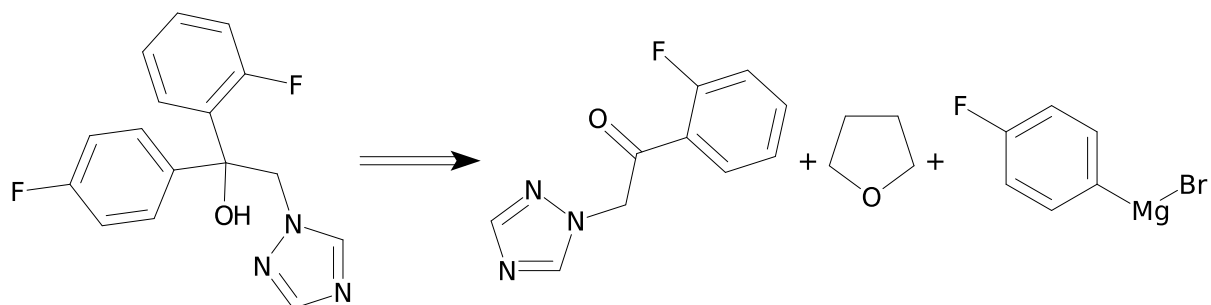

### Step 2

Type: Chloro N-alkylation, Confidence: 0.999

O=C(CCl)c1ccccc1F.c1nc[nH]n1>>O=C(Cn1cncn1)c1ccccc1F

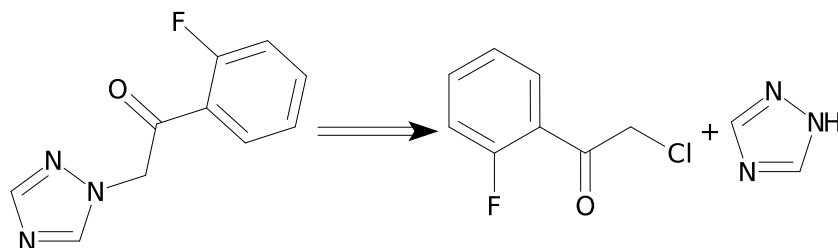

Supplement: Supplementary file 9 [file c2_seq0_final.pdf]
