# Supplementary material for: Unassisted Noise Reduction of Chemical Reaction Data Sets
Source: arXiv:2102.01399 source file (2021-02-02)

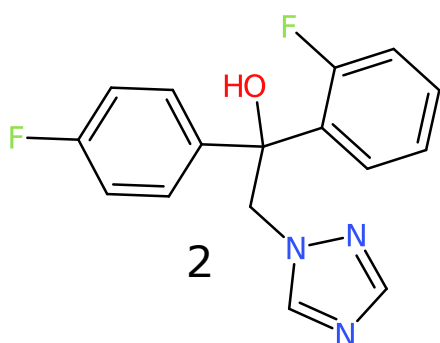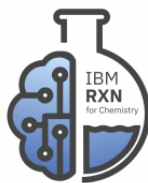

## Information about the retrosynthesis

Created On: 2020-05-18T15:12:49.268000

Model: 2020-04-24

Product: N1(N=CN=C1)CC(C1C=CC=CC=1F)(C1C=CC(F)=CC=1)O

MSSR: 10

FAP: 0.7

MRP: 20

SbP: 2

Available smiles:

Exclude smiles: N(CC(O)(C1=CC=C(F)C=C1)C1C(F)=CC=CC=1)1C=NC=N1,  
N1(N=CN=C1)CC(C1C=CC=CC=1F)(C1C=CC(F)=CC=1)O

Exclude substructures:

Availability pricing threshold: 0

## Sequence 6, Confidence: 0.994

### Step 1

Type: Epoxide + amine coupling, Confidence: 0.994

Fc1ccc(C2(c3ccccc3F)CO2)cc1.CN(C)C=O.O=C([O-])[O-].[K+].[K+].c1nc[nH]n1>>N1(N=CN=C1)CC(C1C=CC=CC=1F)(C1C=CC(F)=CC=1)O

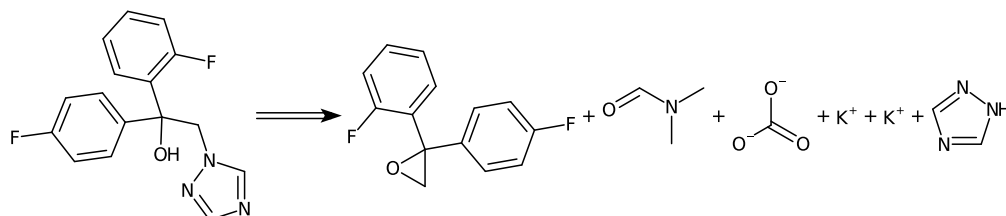

### Step 2

Type: Johnson-Corey-Chaykovsky epoxidation, Confidence: 1.0

CS(C)=O.C[S+](C)(C)=O.[I-].O.O=C(c1ccc(F)cc1)c1ccccc1F.[H-].[Na+].C[S+](C)(C)=O.[I-].[H-].[Na+]>>Fc1ccc(C2(c3ccccc3F)CO2)cc1

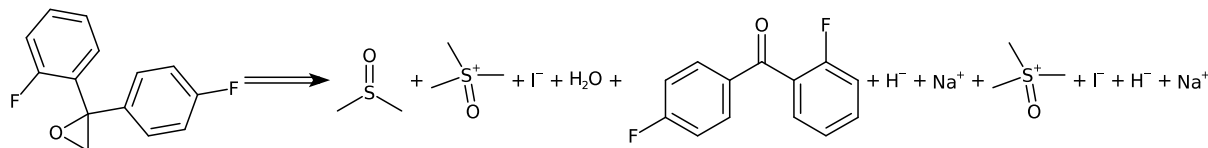

Supplement: Supplementary file 10 [file c2_seq6_final.pdf]
