# Supplementary material for: Unassisted Noise Reduction of Chemical Reaction Data Sets
Source: arXiv:2102.01399 source file (2021-02-02)

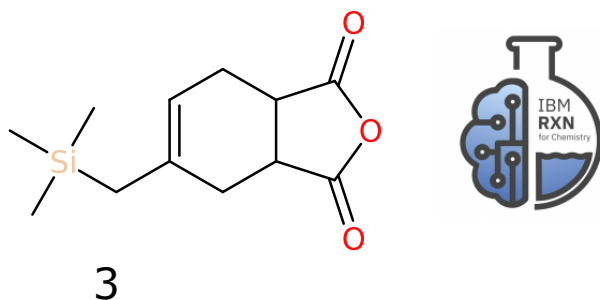

## Information about the retrosynthesis

Created On: 2020-05-18T15:18:52.883000

Model: 2020-04-24

Product: [Si](CC1=CCC2C(C(OC2=O)=O)C1)(C)(C)C

MSSR: 15

FAP: 0.65

MRP: 50

SbP: 3

Available smiles:

Exclude smiles: [Si](CC1=CCC2C(C(OC2=O)=O)C1)(C)(C)C

Exclude substructures:

Availability pricing threshold: 0

## Sequence 0, Confidence: 0.0

Metadata:

Errors: ERROR.No predictions above FAP. Reduce FAP, increase MRP or inspect siblings.

### Step 1

Type: Unrecognized, Confidence: 0.0

C[Si](C)(C)CC1=CCC2C(=O)OC(=O)C2C1>>[Si](CC1=CCC2C(C(OC2=O)=O)C1)(C)(C)C

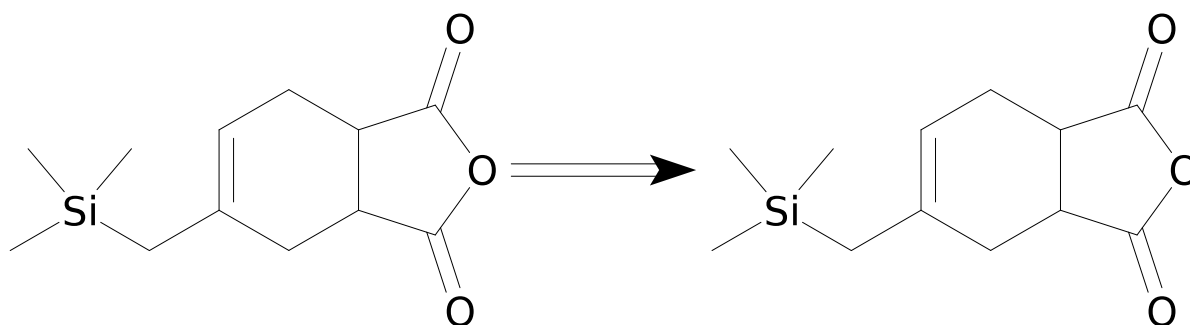

Supplement: Supplementary file 11 [file c3_seq0_final.pdf]
