# Supplementary material for: Unassisted Noise Reduction of Chemical Reaction Data Sets
Source: arXiv:2102.01399 source file (2021-02-02)

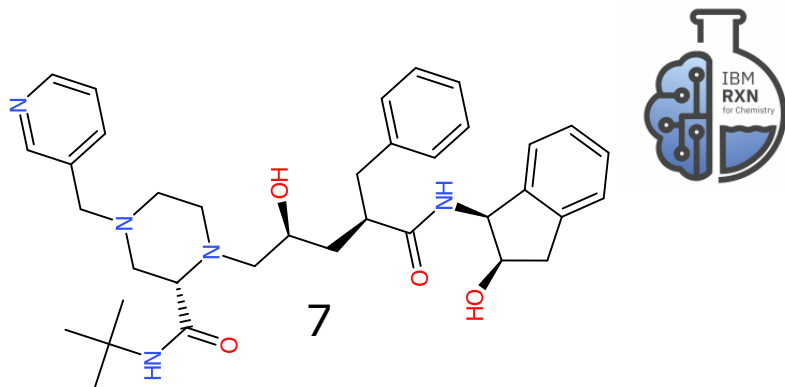

## Information about the retrosynthesis

Created On: 2020-05-29T16:20:31.538000

Model: 2020-04-24

Product: C1C=C2C(C[C@H]([C@H]2NC([C@@H](C[C@@H](CN2[C@H](C(NC(C)(C)C)=O)CN(C(C3C=CC=NC=3)CC2)O)CC2C=CC=CC=2)=O)O)=CC=1

MSSR: 10

FAP: 0.7

MRP: 20

SbP: 2

Available smiles:

Exclude smiles: C1C=C2C(C[C@H]([C@H]2NC([C@@H](C[C@@H](CN2[C@H](C(NC(C)(C)C)=O)CN(C(C3C=CC=NC=3)CC2)O)CC2C=CC=CC=2)=O)O)=CC=1

Exclude substructures:

Availability pricing threshold: 0

## Sequence 0, Conf dence: 0.988

### Step 1

Type: Chloro N-alkylation, Conf dence: 0.988

CC(C)(C)NC(=O)[C@@H]1CNCCN1C[C@@H](O)C[C@@H](Cc1ccccc1)C(=O)N[C@H]1c2cccc  
c2C[C@H]1O.CN(C)C=O.ClCc1ccnc1>>C1=C2C(C[C@H]([C@H]2NC([C@@H](C[C@@H](C  
N2[C@H](C(NC(C)(C)C)=O)CN(CC3C=CC=NC=3)CC2)O)CC2C=CC=CC=2)=O)=CC=1

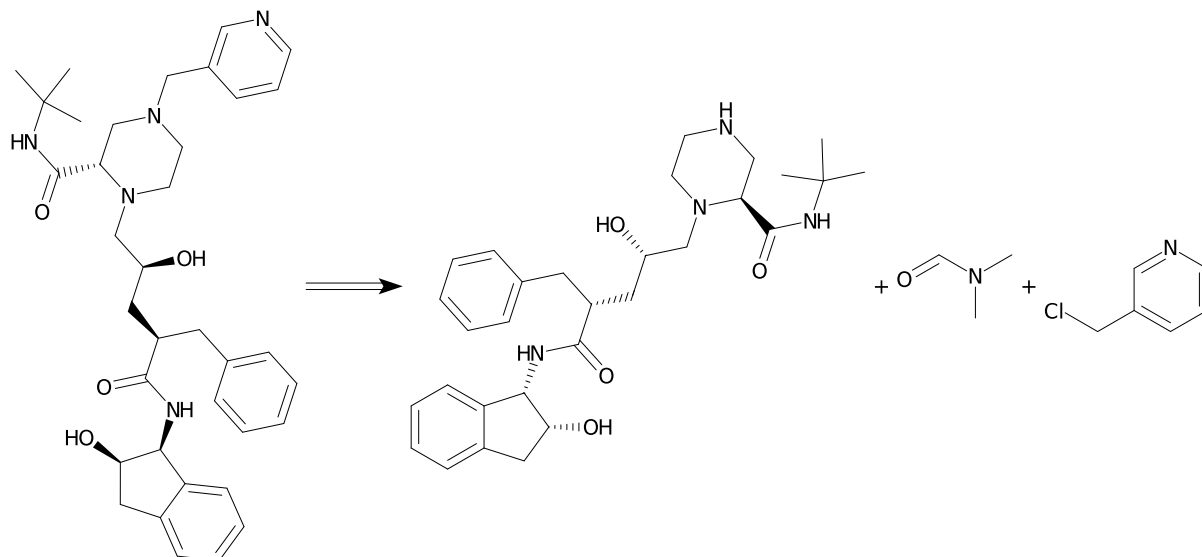

Supplement: Supplementary file 12 [file c7_seq0_final.pdf]
