# Supplementary material for: Unassisted Noise Reduction of Chemical Reaction Data Sets
Source: arXiv:2102.01399 source file (2021-02-02)

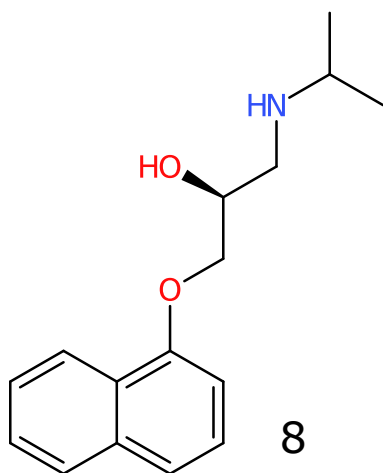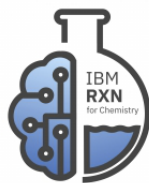

8

## Information about the retrosynthesis

Created On: 2020-05-28T09:06:21.924000

Model: 2020-04-24

Product: C1C2C(=CC=CC=2OC[C@H](CNC(C)C)O)C=CC=1

MSSR: 10

FAP: 0.7

MRP: 20

SbP: 2

Available smiles:

Exclude smiles: C1C2C(=CC=CC=2OC[C@@H]2CO2)C=CC=1,

C1C2C(=CC=CC=2OC[C@H](CNC(C)C)O)C=CC=1

Exclude substructures:

Availability pricing threshold: 0

## Sequence 0, Confidence: 0.996

### Step 1

Type: Epoxide + amine coupling, Confidence: 1.0

c1ccc2c(OC[C@@H](CO3)cccc2c1)CC(C)N.CO>>C1C2C(=CC=CC=2OC[C@H](CNC(C)C)O)C=CC=1

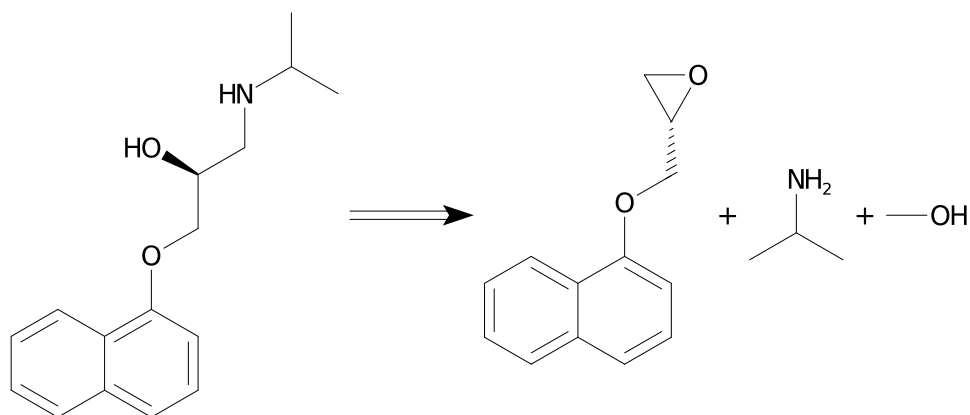

### Step 2

Type: Unrecognized, Confidence: 0.996

CN(C)C=O.O=[N+]([O-])c1cccc(S(=O)(=O)OC[C@@H](CO2)c1)Oc1cccc2ccccc12.[NaH]>>c1ccc2c(OC[C@@H](CO3)cccc2c1)CC(C)N.CO>>C1C2C(=CC=CC=2OC[C@H](CNC(C)C)O)C=CC=1

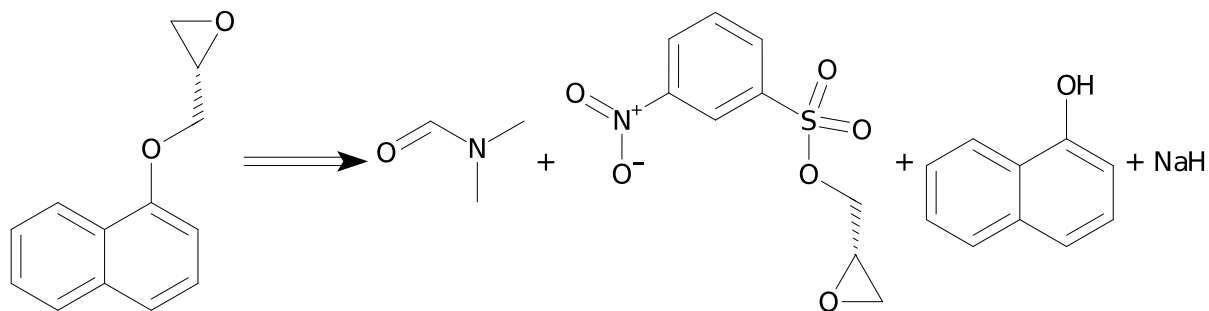

Supplement: Supplementary file 13 [file c8_seq0_final.pdf]
